# Supplementary material for: A Deep Perceptual Measure for Lens and Camera Calibration
Source: arXiv:2208.12300 source file (2023-07-26)
Supplement: Supplementary file 1 [file sec_appendix.tex]

\begin{itemize}
    \item more results on horizon estimation (fig. 2) [JF]
    \item derivations of equations for intrinsic parameters (end of sec. 3.2) [Yan]
    \item camera setup for the comparison with metrology methods (sec 5.3, table 2) [Yan]
    \item estimated parameters for the comparison with metrology methods (sec 5.3, table 2) [Yan]
    \item smoothed guided backprop (fig. 4) [JF]
    \item combinations of parameters (fig. 8) [Yan]
    \item undistortion results (fig. 9) [JF]
    \item virtual object insertions (fig. 12)
    \item geometrically consistent object transfer (ancienne figure). 
    \item human perceptual loss figures (dominique's figures) [JF]
\end{itemize}

\subsection{Rescaling image}

\subsubsection{Pinhole and focal length $f$}
In the following, we consider only the pinhole model, i.e. no distortion $\xi$.

We answer the question: when we resize an image to the CNN resolution, how does it modify the focal length $f$?\\

Answer: By resizing the image by $s$, the new focal length is $f/s$. Obvious :-)

Intrinsic calibration matrix:
\[
K
=
\begin{bmatrix}
    f & 0 & u_0 \\
    0 & f & v_0 \\
    0 & 0 & 1
\end{bmatrix}
\]

In full resolution, a world point $(X,Y,Z)$ is projected to the image point in pixels:
\[
\begin{bmatrix}
    x \\
    y \\
    w
\end{bmatrix}
=
K
\begin{bmatrix}
    X \\
    Y \\
    Z
\end{bmatrix}
\]
i.e.
\[
\begin{bmatrix}
    x \\
    y
\end{bmatrix}
=
\begin{bmatrix}
    \frac{fX}{Z} +u_0 \\
    \frac{fY}{Z} +v_0
\end{bmatrix}
\]

When the image is scaled by $s$, then this pixel is now at $(x',y')=(x/s,y/s)$ and the image center is at $(u_0/s,v_0/s)$. Let's note $f'$ the ``new" focal length and
\[
K'
=
\begin{bmatrix}
    f' & 0 & u'_0 \\
    0 & f' & v'_0 \\
    0 & 0 & 1
\end{bmatrix}
=
\begin{bmatrix}
    f' & 0 & u_0/s \\
    0 & f' & v_0/s \\
    0 & 0 & 1
\end{bmatrix}
\]

Thus
\[
\begin{bmatrix}
    x' \\
    y'
\end{bmatrix}
=
\begin{bmatrix}
    \frac{f'X}{Z} +u'_0 \\
    \frac{f'Y}{Z} +v'_0
\end{bmatrix}
=
\begin{bmatrix}
    \frac{f'X}{Z} +u_0/s \\
    \frac{f'Y}{Z} +v_0/s
\end{bmatrix}
\]

Thus, to get $x/s=\frac{f'X}{Z}+u_0/s$ for all $X$, and given that $x=\frac{fX}{Z} +u_0$ , we need $f'=f/s$.

In other terms, resizing the image by the scale $s$ essentially rescales (inherently/intrinsically) the value of the focal length $f$ by $s$. Obvious :-)

\subsubsection{Sphere model: focal length $f$ and distortion $\xi$}

As a generalization of the previous question: when we resize an image to the CNN resolution, how does it modify the focal length $f$ and the distortion parameter $\xi$?\\

From World/Sphere points to image points:
\begin{equation}
%\resizebox{0.91\hsize}{!}{%
\resizebox{0.91\hsize}{!}{$\mathbf{p} =(x,y)=\left( \frac{Xf}{\xi\sqrt{X^2+Y^2+Z^2}+Z}+u_0,\frac{Yf}{\xi\sqrt{X^2+Y^2+Z^2}+Z}+v_0 \right),$
}
\label{SphProj1}
\end{equation}

From image point to sphere point:
\begin{equation}
 \mathbf{P_s} = (\omega \hat{x}, \omega \hat{y}, \omega - \xi) ~~~~~ \mbox{with~~~~~} \omega = \frac{\xi + \sqrt{1 + (1-\xi^2)(\hat{x}^2+\hat{y}^2)}}{\hat{x}^2+\hat{y}^2+1},
  \label{Eq::backPro}
\end{equation}
and
 \begin{equation}
 \begin{bmatrix}
 \hat{x},
  \hat{y},
 1
 \end{bmatrix}^{T}\simeq \mathbf{K}^{-1}\mathbf{p}
 ~~~~~ \mbox{where~~~~~} 
     \mathbf{K}=\begin{bmatrix}
f & 0 & u_0 \\
0 & f & v_0 \\
0 & 0 & 1 
 \end{bmatrix}.
 \end{equation}
 
From World/Sphere points to image points:
\begin{equation}
%\resizebox{0.91\hsize}{!}{%
\resizebox{0.91\hsize}{!}{$\mathbf{p} =(x,y)=\left( \frac{Xf}{\xi\sqrt{X^2+Y^2+Z^2}+Z}+u_0,\frac{Yf}{\xi\sqrt{X^2+Y^2+Z^2}+Z}+v_0 \right),$
}
\label{SphProj1}
\end{equation}

When the image is scaled by $s$, then this pixel is now at $(x',y')=(x/s,y/s)$ and the image center is at $(u_0/s,v_0/s)$. Let note the unknown resulting focal length $f'$ and distortion parameter $\xi'$. 
 
Thus we have
\begin{align}
\mathbf{p'} &= (x',y')=(x/s,y/s) \\
&= \left( \frac{Xf'}{\xi'\sqrt{X^2+Y^2+Z^2}+Z}+u'_0,\frac{Yf'}{\xi'\sqrt{X^2+Y^2+Z^2}+Z}+v'_0 \right) \\
&= \left( \frac{Xf'}{\xi'+Z}+u'_0,\frac{Yf'}{\xi'+Z}+v'_0 \right) \textrm{ since points on sphere}\\
&= \left( \frac{Xf'}{\xi'+Z}+u_0/s,\frac{Yf'}{\xi'+Z}+v_0/s \right)
\label{SphProj1}
\end{align}
 
Summary so far: we have 
\begin{equation}
\mathbf{p} = (x,y) = \left( \frac{Xf}{\xi+Z}+u_0,\frac{Yf}{\xi+Z}+v_0 \right)
\label{SphProj1}
\end{equation}
and
\begin{equation}
\mathbf{p'} = (x',y') = \left( \frac{Xf'}{\xi'+Z}+u_0/s,\frac{Yf'}{\xi'+Z}+v_0/s \right)
\label{SphProj1}
\end{equation}

To have $(x',y')=(x/s,y/s)$ for all $X,Y,Z$,
we need
\begin{equation}
\left( \frac{Xf'}{\xi'+Z},\frac{Yf'}{\xi'+Z}\right)
=
\left( \left(\frac{Xf}{\xi+Z}\right) \bigg/ s, \left(\frac{Yf}{\xi+Z}\right) \bigg/ s \right)
\label{SphProj1}
\end{equation}

Therefore one solution is to have $f'=f/s$ and $\xi'=\xi$.

Important note: maybe there are also other solutions.

Figure~\ref{fig:resizing_sphmodel}: left  obtained by $H\times W$, with $f$ and $\xi$, and then resizing by the scale $s$. Right: obtained by $(H/s) \times (W/s)$, with $f/s$ and $\xi$. The two images are the same

\begin{figure}[t]
	\vspace{-1mm}
	\centering
	\subfigure[]{\includegraphics[width=0.48\linewidth]{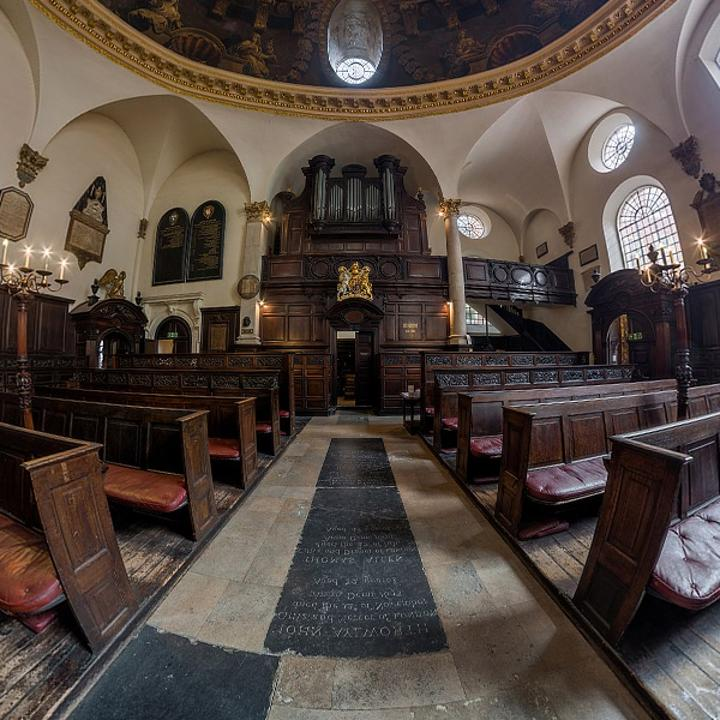}}
	\subfigure[]{\includegraphics[width=0.48\linewidth]{figures/exp_resizing/Exp2.jpg}} 
	\vspace{-0mm}
	\caption{Testing the intrinsic parameters w.r.t. resizing. The two images look the same, so our derivations are correct. See main text.}
	\label{fig:resizing_sphmodel}
% 	\vspace{-4mm}
\end{figure}
 
\subsection{Given $(u_0,v_0)$ (i.e. thus the image size $H \times W$) and $f$ and $\xi$, compute the horizontal field of view}

TODO: add figures

Image size: $H \times W$. Camera center in the middle: $(u_0,v_0)=(W/2,H/2)$.

Project the center point $(u_0,v_0)$ onto the sphere. Two steps. First apply $K^{-1}$, and obtain $(0,0,1)$. 
Second, apply the projection function: obtain $P_0=(0,0,1)$.

Given the ``left point" $(0,H/2)=(0,v_0)$, project it onto the sphere. Two steps. First apply $K^{-1}$, and obtain $(\hat{x},\hat{y},\hat{w})=(-u_0/f,0,1)$. 
Second, apply the projection function: obtain $P_s=\left(\omega \hat{x}, 0 , \frac{\xi+\sqrt{1+(1-\xi^2)\hat{x}^2}}{\hat{x}^2 +1} - \xi\right)$.

Let's write $FOV=\alpha$

$\frac{\alpha}{2}=\arccos(P_0 \cdot P_s)=\arccos{\left(\frac{\xi+\sqrt{1+(1-\xi^2)\hat{x}^2}}{\hat{x}^2+1} -\xi \right)}$ with $\hat{x}=-u_0/f$.

i.e. the field of view is $\alpha = 2 \arccos(P_0 \cdot P_s)$

\begin{equation*}
FOV=2\arccos{\left(\frac{\xi+\sqrt{1+(1-\xi^2)\hat{x}^2}}{\hat{x}^2+1} - \xi\right)}
\end{equation*}
with $\hat{x}=-u_0/f$.

\textbf{Note:} by looking at this final equation, we can see that, if $u_0$ (i.e. image size) and $f$ are scaled by the same value $s$, then the FOV does not change (with $\xi$ fixed).

\subsection{Given $(u_0,v_0)$ (i.e. thus the image size $H \times W$) and (horizontal) FOV and $f$ (resp. $\xi$), compute $\xi$ (resp. $f$}

TODO: add figure

For the horizontal field of view, the spherical points are on the horizon plane ($X-Z$ plane), i.e. on $Y=0$.

$P_0$ is known: $(0,0,1)$, see above section.

$\sin(\alpha/2)=\frac{-X}{1}=X$, thus $X=-\sin(\alpha/2)$.

We have $X^2+Z^2=1$, thus $Z=\pm \sqrt{1-X^2}$.
In summary, given the FOV $\alpha$, we can get $X$ and $Z$.

$p=(x,y)=\left(\frac{X f}{\xi \cdot 1 + Z} + u_0 , \frac{Y f}{\xi \cdot 1 + Z} + v_0\right)$.

$p=(x,y)$ must be equal to $(0,v_0)$.

For $y$: We have $Y=0$ since on the horizon plane (see above), therefore $\frac{Y f}{\xi \cdot 1 + Z} + v_0=0+v_0=v_0$, which is good.

For $x$, we must have $\frac{X f}{\xi \cdot 1 + Z} + u_0 = 0$.

Given $\xi$, this leads to $f=-u_0(\xi+Z)/X$, where $X$ and $Z$ are known given the FOV $\alpha$.

Given $f$, this leads to $\xi=\frac{Xf+u_0Z}{-u_0}$, where $X$ and $Z$ are known given the FOV $\alpha$.

\subsection{Given $(u_0,v_0)$ (i.e. thus the image size $H \times W$) and  $f$, compute midpoint $b_p$}

Image size $H \times W$, camera center in the middle $(u_0, v_0) = (W/2, H/2)$.

Project the center $(u_0, v_0)$ on the sphere, first by applying $K^{-1}$ to get $(\hat{x}, \hat{y}, 1)=(0,0,1)$, then by projecting on the sphere to get $P_S = (0,0,1)$. Rotate the point on the sphere by a elevation angle $\theta$ to get
\begin{align*}
P_s
    &=
    \begin{bmatrix}
    1& 0& 0\\
    0 & \cos\theta & -\sin\theta\\
    0 & \sin\theta & \cos\theta
    \end{bmatrix}
    \begin{bmatrix}
    0\\0\\1
    \end{bmatrix}\\
    &=\begin{bmatrix}
    0\\-\sin\theta\\\cos\theta
    \end{bmatrix}
\end{align*}

Project on the image plane to get $(x, y)=\left(u_0, \frac{-f\sin\theta}{\xi+\cos\theta}+v_0\right)$. The midpoint is thus

\begin{align*}
    b_p = -f\frac{\sin\theta}{\xi+\cos\theta}+v_0
\end{align*}

If we set $\xi=0$, we get $b_p=-f\tan\theta + v_0$, the usual equation.

\resizebox{\linewidth}{!}{
\begin{tabular}{rlrrr}
%\cline{2-5}
& \textbf{Method}         & $f$    & \textbf{distortion}                  &  \begin{tabular}{@{}r@{}}\textbf{avg err} \vspace{-0.5em} \\ \footnotesize (px)\end{tabular} \\ %\hline %\hline
\multicolumn{1}{c}{\multirow{6}{*}{\vspace{4mm} \begin{tabular}{ c }
  Avenir 2.8mm \\
  \includegraphics [width=0.18\linewidth]{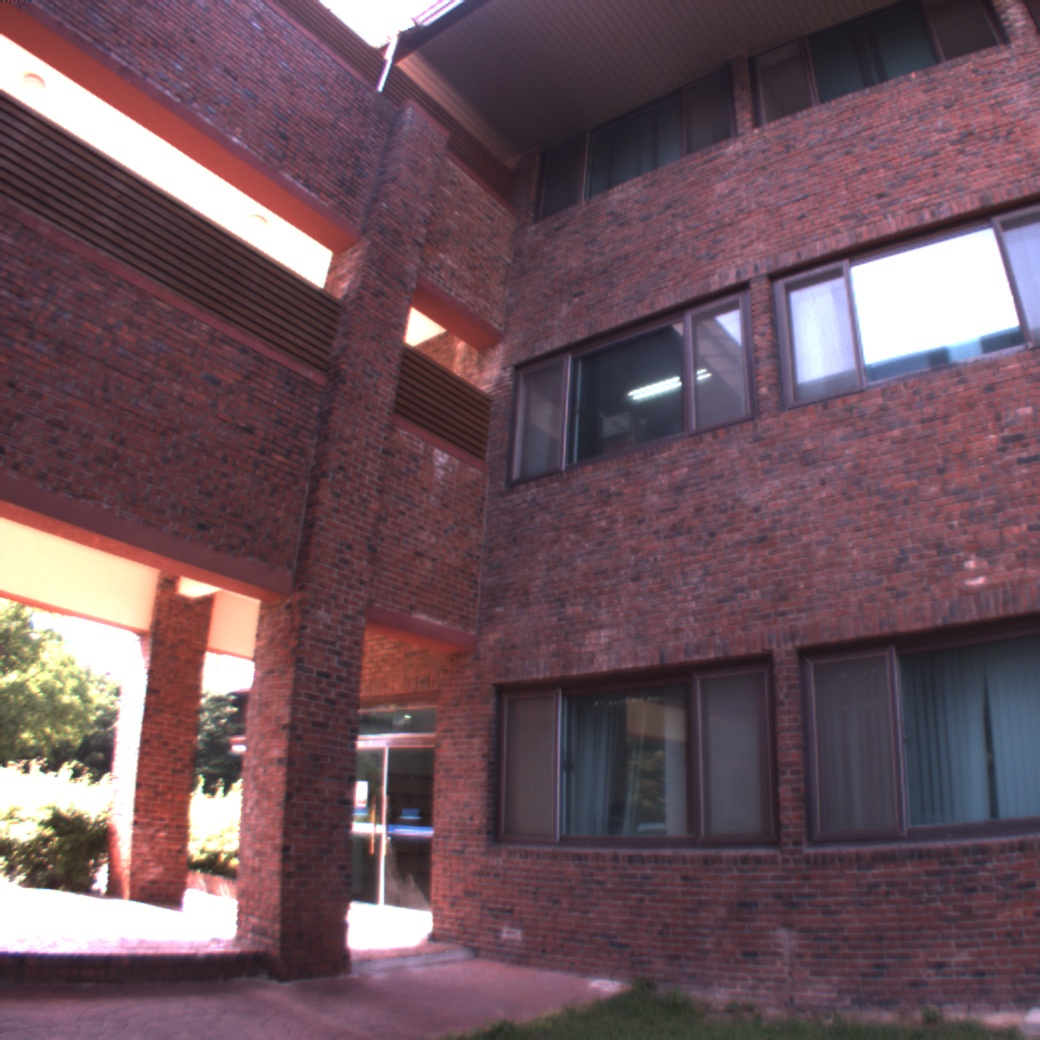}
\end{tabular}}} & Ours           & 1288  & 0.69490                            & 0.63578            \\ %\cline{2-5} 
\multicolumn{1}{l}{}                            & Mei~\cite{mei2007single}            & 1973 & 1.48                         & 0.12           \\ %\cline{2-5} 
\multicolumn{1}{l}{}                            & Division~\cite{fitzgibbon2001simultaneous} & N/A %331 
& N/A %0.00, 0.00, 0.00, 0.00 
& N/A%98.19 
\\
%\cline{2-5} 
\multicolumn{1}{l}{}                            & Brown~\cite{Zhang:TPAMI:00}   & 796   & -0.30, 0.17, -0.00, -0.00, -0.07 & 0.20           \\ %\cline{2-5} 
\multicolumn{1}{l}{}                            & Scaramuzza~\cite{Scaramuzza:IROS:06}     &  788   &   -788.50, 0,  $3.55^{-4}$,  $2.11^{-7}$,  $-2.62^{-10}$                         & 1.01            \\ \rule{0pt}{3ex}%\rule[-0.9ex]{8pt}{0pt} %\hline
\multicolumn{1}{c}{\multirow{6}{*}{ 
\vspace{4mm} \begin{tabular}{ c }
  Avenir 4mm \\
  \includegraphics [width=0.18\linewidth]{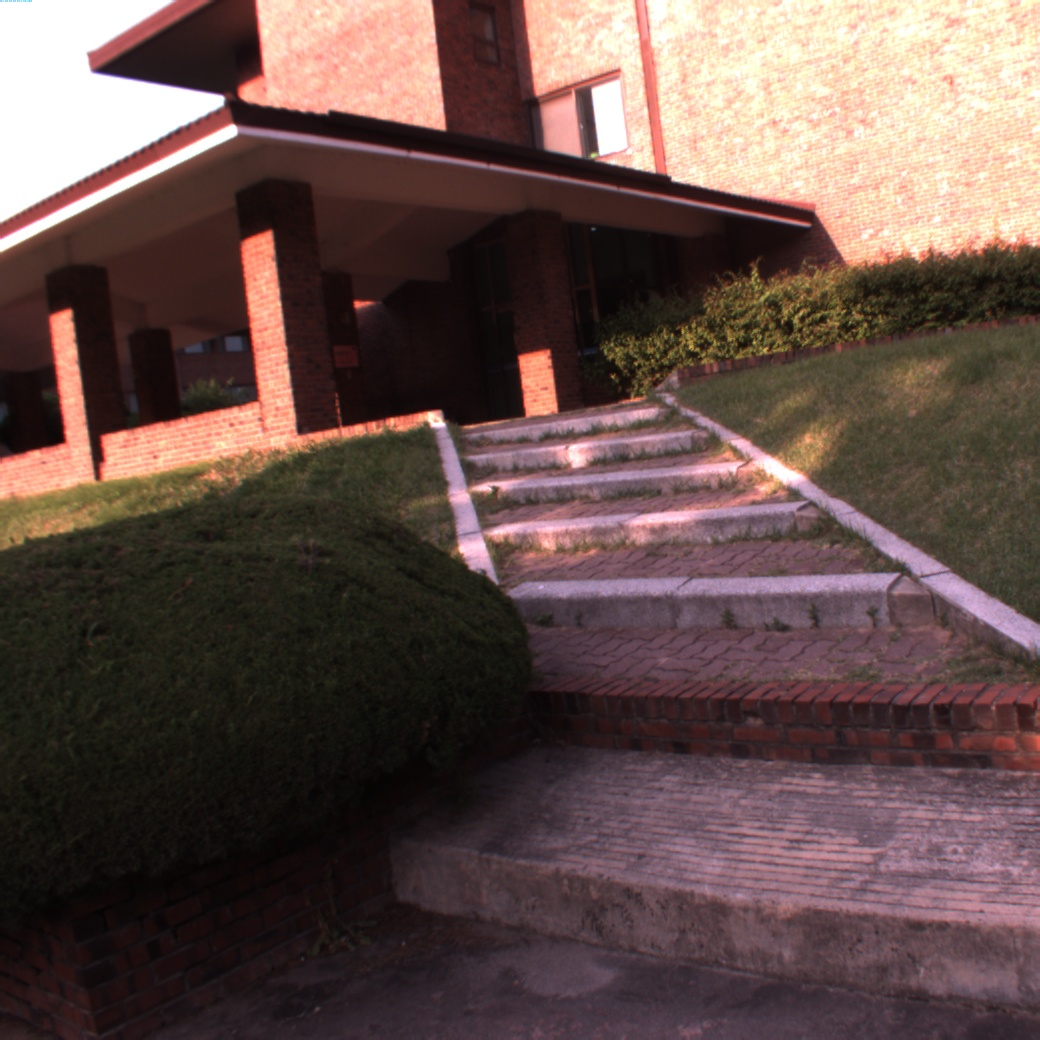}
\end{tabular}}} & Ours           & 1485  & 0.3681                            & 0.57        \\ %\cline{2-5} 
\multicolumn{1}{l}{}                            & Mei            & 2270  & 0.97                            & 0.13        \\ %\cline{2-5} 
\multicolumn{1}{l}{}                            & Division & N/A%331 
& N/A %0.00, 0.00, 0.00, 0.00
& N/A % 139.05
\\
%\cline{2-5} 
\multicolumn{1}{l}{}                            & Brown   & 1158 & -0.27, 0.28, 0.00, 0.00, -0.21   & 0.29          \\ %\cline{2-5} 
\multicolumn{1}{l}{}                            & Scaramuzza     & 1157     &  -1157, 0.00, $2.89^{-4}$, $-2.45^{-7}$, $1.79^{-10}$
                               & 0.54          \\  \rule{0pt}{3ex} %\hline
\multicolumn{1}{c}{\multirow{6}{*}{\vspace{4mm} \begin{tabular}{ c }
  GoPro \\
  \includegraphics [width=0.31\linewidth]{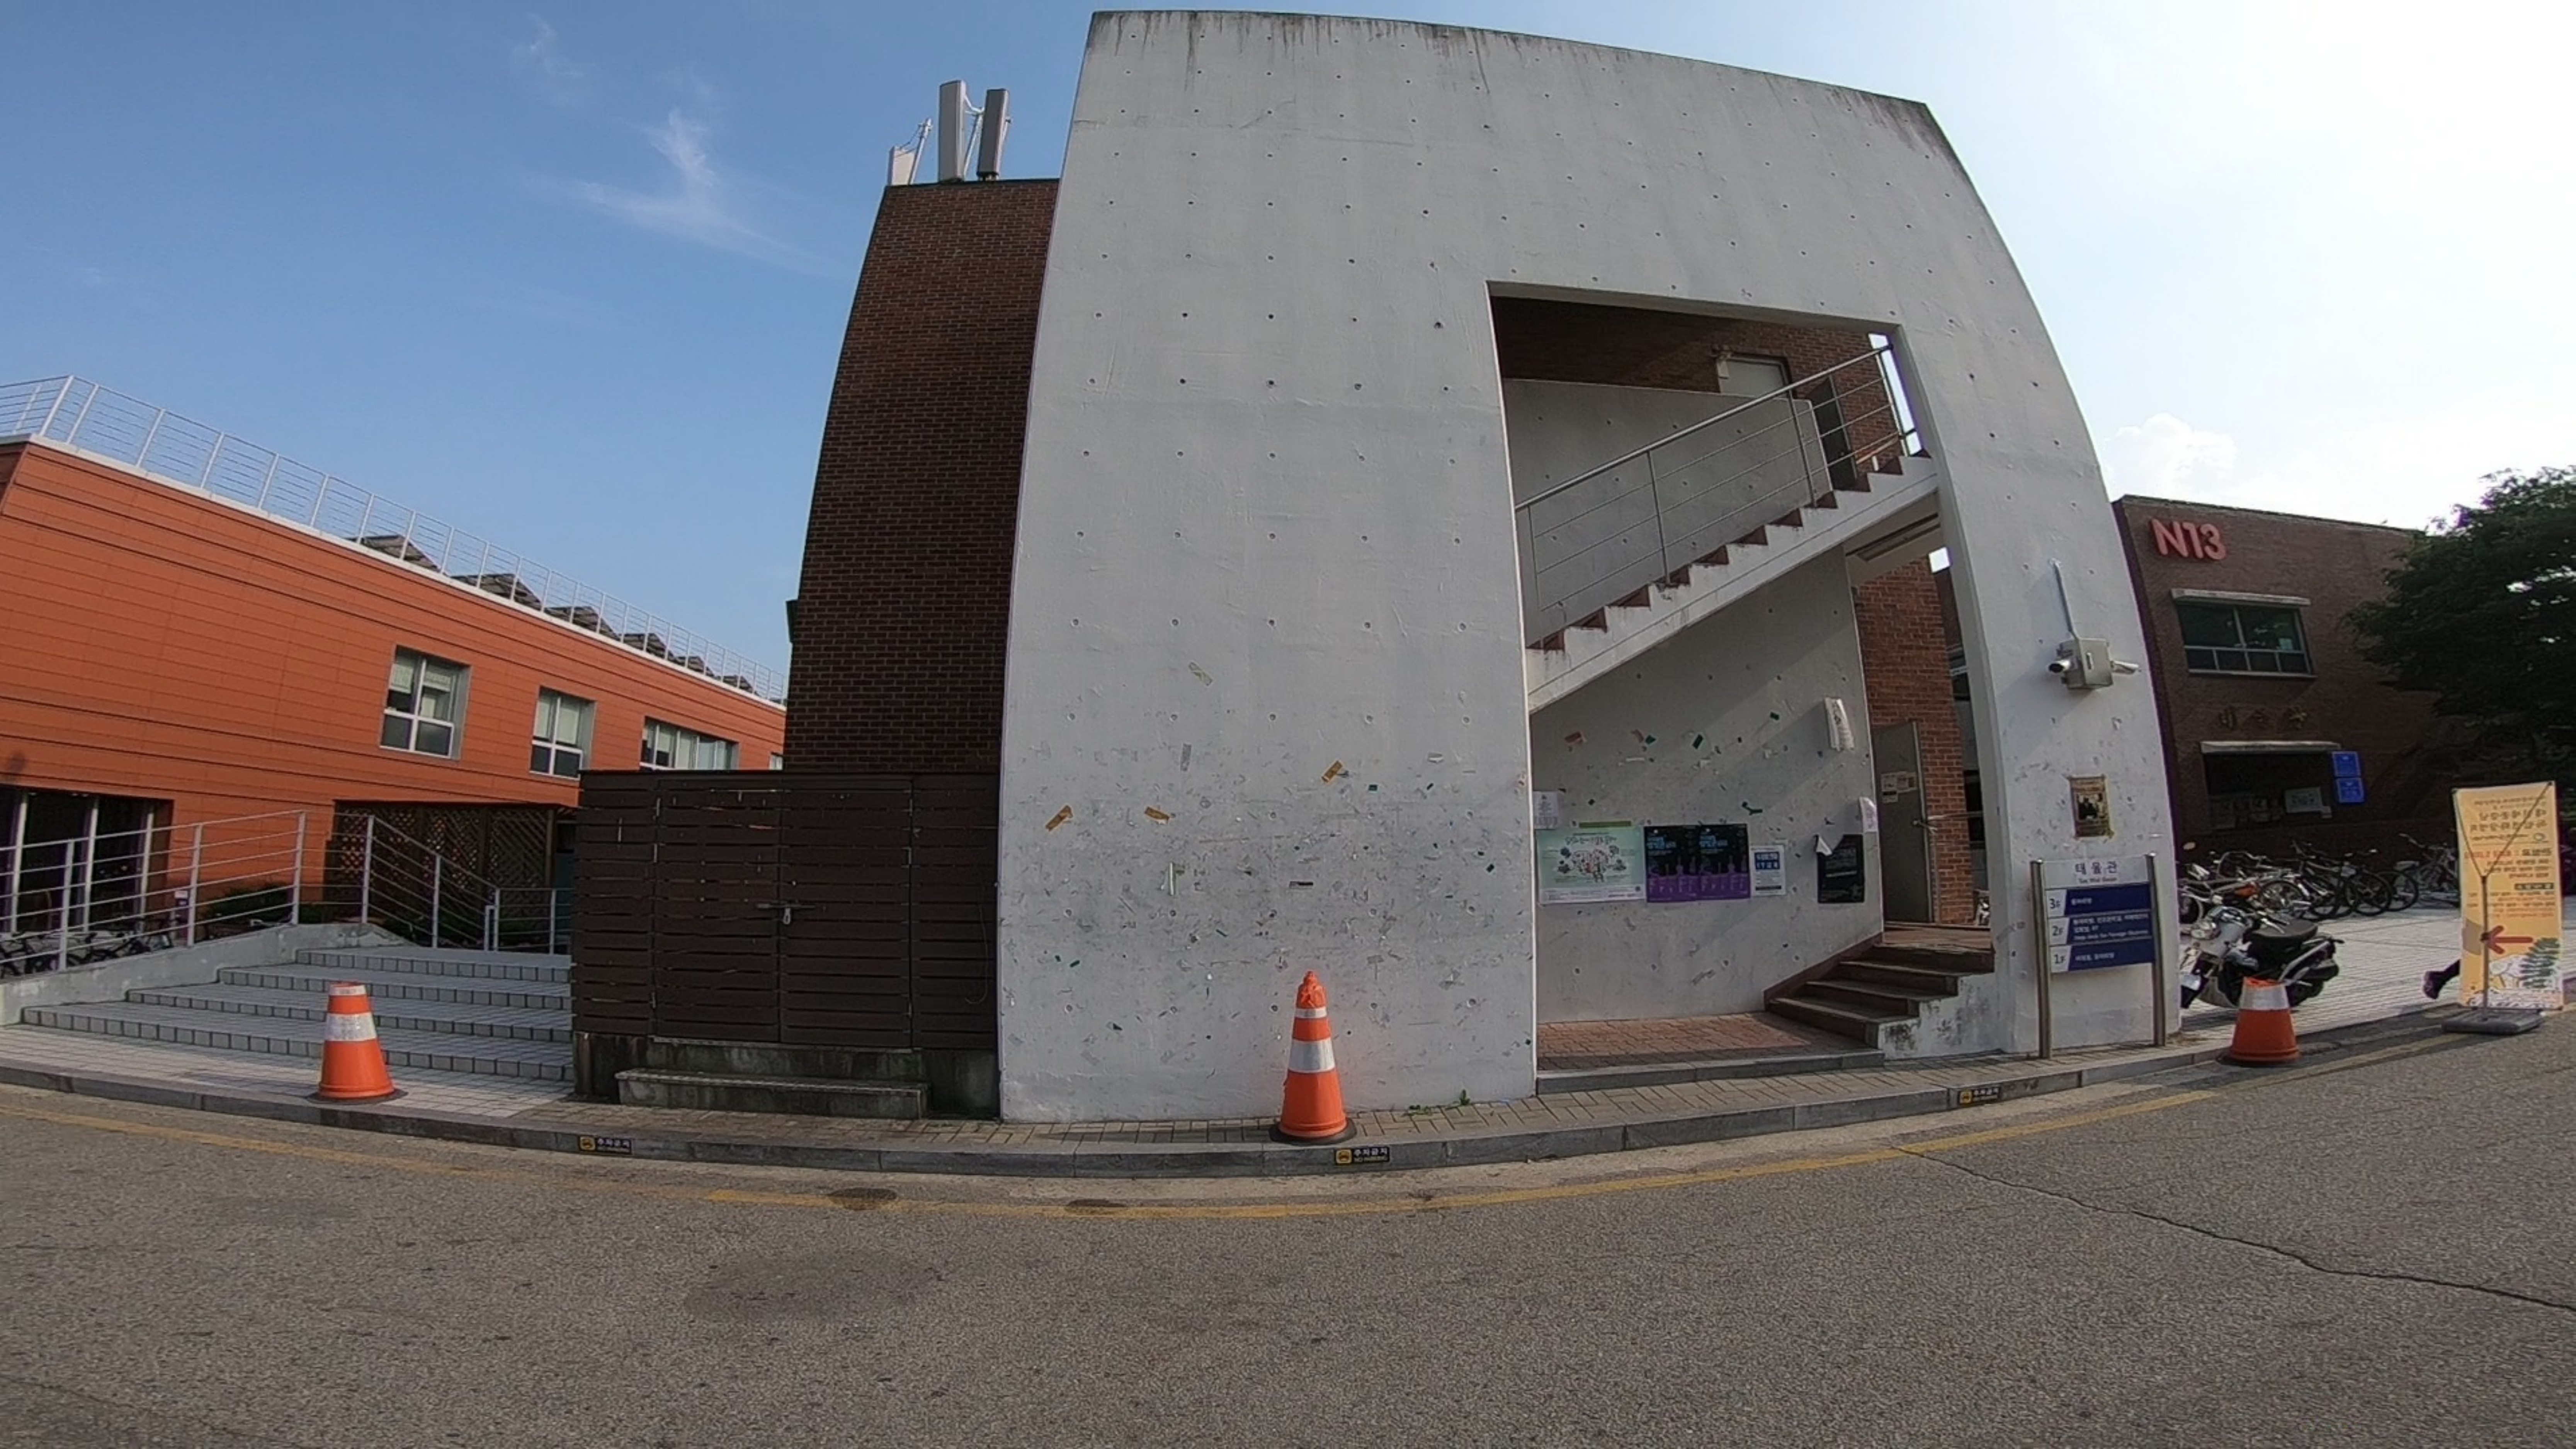}
\end{tabular}}}      & Ours           & 1182  & 0.82                            & 1.11        \\ %\cline{2-5} 
\multicolumn{1}{l}{}                            & Mei            & 1561 &  1.28                            & 0.12        \\ %\cline{2-5} 
\multicolumn{1}{l}{}                            & Division & 787  & 0.15, -0.77, 1.61, -0.98        & 0.7           \\ %\cline{2-5} 
\multicolumn{1}{l}{}                            & Brown   & N/A    & N/A                        & N/A              \\ %\cline{2-5} 
\multicolumn{1}{l}{}                            & Scaramuzza     & 791    &    -791.4, 0.00, 0.00, $-1.12^{-6}$, $3.10^{-10}$                            & 0.82           \\ \rule{0pt}{3ex} %\hline
\multicolumn{1}{c}{\multirow{6}{*}{\vspace{4mm} \begin{tabular}{ c }
  Fisheye \\
  \includegraphics [width=0.18\linewidth]{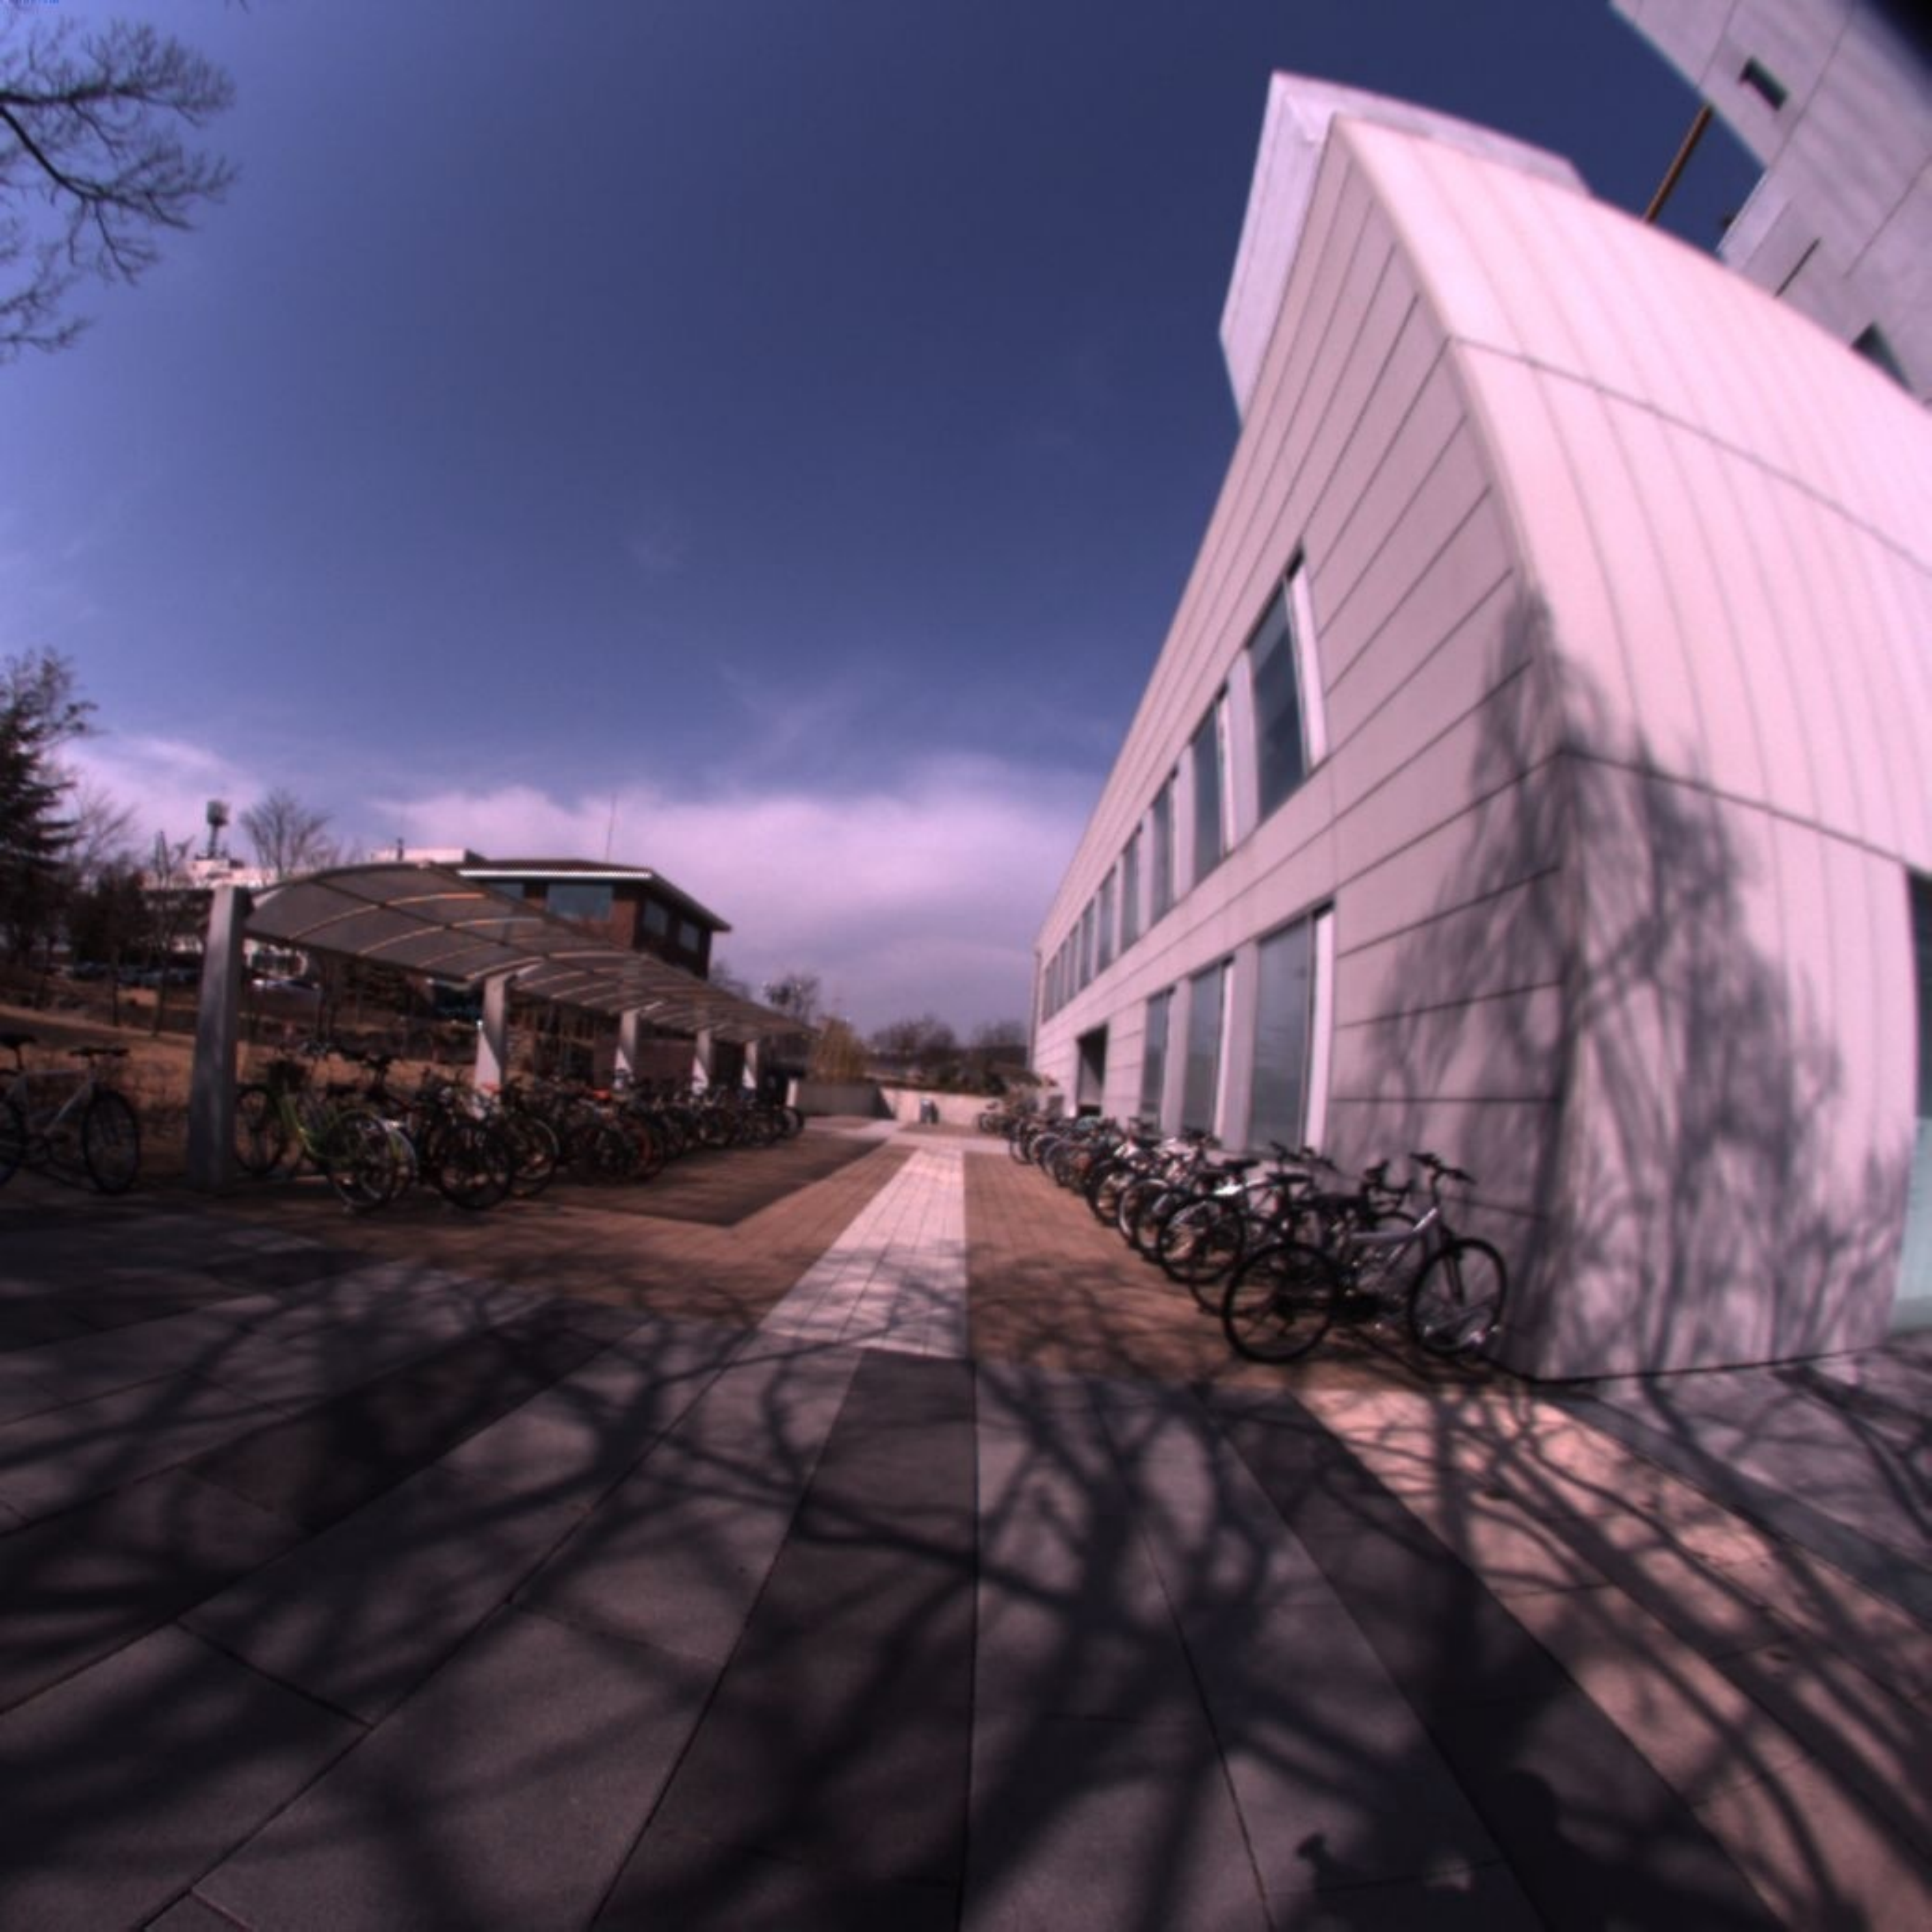}
\end{tabular}}}    & Ours           & 850  &  0.85                            & 1.25           \\ %\cline{2-5} 
\multicolumn{1}{l}{}                            & Mei            & 1351 &  1.79                            & 0.10          \\ %\cline{2-5} 
\multicolumn{1}{l}{}                            & Division & 488  & -0.09, 0.65, -1.79,  1.13        &  1.05           \\ %\cline{2-5} 
\multicolumn{1}{l}{}                            & Brown   & N/A     & N/A                              & N/A              \\
%\cline{2-5} 
\multicolumn{1}{l}{}                            & Scaramuzza     &   487    & -487.7, 0, $8.18^{-4}$,  $-4.39^{-7}$, $4.32^{-10}$                                & 1.48            \\ %\hline 
\end{tabular}
}
\label{Tab::CaMcal}
\vspace{-2mm}
\end{table}

\subsection*{Geometrically-consistent object transfer}
\yhg{reword, this is verbatim the paper paragraph} Transferring objects from one image to another requires matching the camera parameters. While previous techniques required the use of objects of known height in the image in order to infer camera parameters~\cite{lalonde-siggraph-07}, our approach estimates them from the image itself, and can be used to realistically transfer objects from one image to another, as shown in the supp. material. 

\begin{figure}[!t]
\centering
\includegraphics[width=0.7\linewidth]{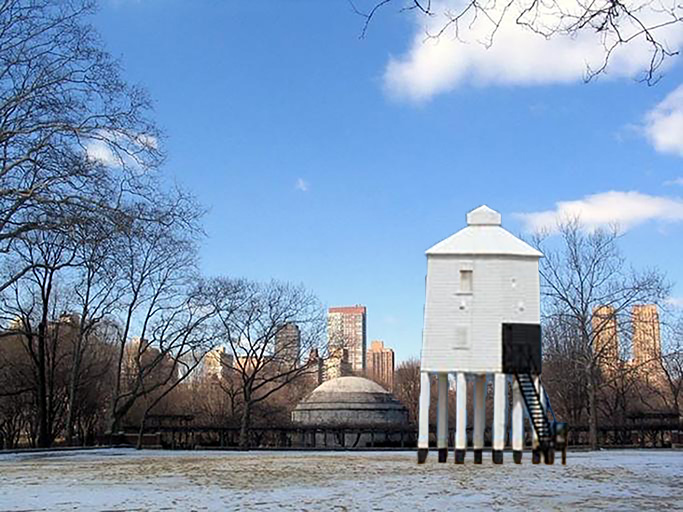}
\caption{The water tower from fig.~\ref{fig:applications_retrieval} pasted onto an image with an automatically detected similar horizon line. Note how the perspective looks right without modification.\vspace{-0.7em}}
\label{fig:applications_2d_compositing}
\vspace{-0.5em}
\end{figure}
